# Supplementary material for: Decidability of the interval temporal logic ABBar over the natural numbers
Source: arXiv:0912.3429 source file (2010-02-03)
Supplement: Supplementary file 1 [file appendix.tex]

\section{Appendix}\label{app:appendix}

In this appendix, we report some complete proofs that have been omitted in the previous sections.
Moreover, we describe an EXPSPACE (optimal) procedure that decides satisfiability of $\ABB$.

\subsection{Proof of Lemma \ref{lemma:entanglement}}\label{app:entanglement}

\smallskip\noindent
{\bf Lemma \ref{lemma:entanglement}.}
\emph{
If $F\dep{A}H$ and $G\dep{B}H$ hold for some atoms $F,G,H$, then $F\dep{A}G$ holds as well.
}
\medskip

\begin{proof}
Suppose that $F\dep{A}H$ and $G\dep{B}H$ hold for some atoms $F,G,H$. By applying the definitions
of the relations $\dep{A}$ and $\dep{B}$, we immediately obtain:
$$
\begin{array}{rcll}
  \req_A(F) &=& \obs(H) \,\cup\, \req_B(H) \,\cup\, \req_{\bar{B}}(H) & \quad\text{(since $F\dep{A}H$)}  \s1 \\
            &=& \obs(G) \,\cup\, \req_B(G) \,\cup\, \req_{\bar{B}}(G) & \quad\text{(since $G\dep{B}H$)}.
\end{array}
$$
This shows that $F\dep{A}G$.
\end{proof}

\subsection{Proof of Theorem \ref{th:contraction_infinite}}\label{app:contraction_infinite}

\smallskip\noindent
{\bf Theorem \ref{th:contraction_infinite}.}
\emph{
An $\ABB$-formula $\varphi$ is a satisfied by an infinite interval structure iff it is featured 
by a periodic compass structure with threshold $\til{y}_0<2^{2^{7\len{\varphi}}}$ and period 
$\til{y}<2\len{\varphi}\cdot 2^{2^{7\len{\varphi}}}\cdot 2^{2^{7\len{\varphi}}}$. 
}
\medskip

\begin{proof}
One direction is trivial. We prove the other one (``only if'' part). Suppose that $\varphi$ 
is satisfied by an infinite interval structure $\cS$. By Proposition \ref{prop:compassstructure}, 
there is an infinite compass structure $\cG$ that features $\varphi$. Below, we show how to turn
$\cG$ into a periodic compass structure $\cG'$ that still features $\varphi$ and whose threshold 
and period satisfy the bounds given by the theorem.

\smallskip\noindent
\textsc{Threshold $\til{y}_0$.\;\;} 
Since $\cG$ is infinite, we know that there exist infinitely many rows $y_0,y_1,y_2,...$ 
such that $\shading_\cG(y_i)=\shading_\cG(y_j)$ for every pair of indices $i,j\in\bbN$. We 
define $\til{y}_0$ as the least of all such rows. By simple counting arguments, we have that 
$\til{y}_0<2^{2^{7\len{\varphi}}}$.

\begin{figure}[!tb]
\centering
\includegraphics[scale=0.95]{draft.3}
\caption{A set $\img_y(f)$ of rows that fulfill all requests at row $\til{y}_0$.}
\label{fig:gaps}
\end{figure}
\smallskip\noindent
\textsc{Period $\til{y}$.\;\;} 
Since $\cG$ is a (fulfilling) compass structure, there is a function $f$ that maps any point $p=(x,\til{y}_0)$,
any relation $R\in\{A,\bar{B}\}$, and any request $\alpha\in\req_R\bigl(\cL(p)\bigr)$ to a point $p'=f(p,R,\alpha)$ 
such that $p \;R\; p'$ and $\alpha\in\obs\bigl(\cL(p')\bigr)$. Let $f$ be one such function. We denote by $\img(f)$ 
the image set of $f$, namely, the set of all points of the form $p'=f(p,R,\alpha)$, with 
$p=(x,\til{y}_0)$, $R\in\{A,\bar{B}\}$, and $\alpha\in\req_R\bigl(\cL(p)\bigr)$. Moreover, we denote by $\img_y(f)$ the 
projection of $\img(f)$ on the $y$-component. Intuitively, $\img_y(f)$ is a minimal set of rows that fulfill 
all $A$-requests and all $\bar{B}$-requests of atoms along the row $\til{y}_0$ in $\cG$ (see, for instance, Figure
\ref{fig:gaps}). Clearly, $\min\bigl(\img_y(f)\bigr)>\til{y}_0$ and $\img_y(f)$ contains at most $2\len{\varphi}\cdot\til{y}_0$ 
(possibly non-contiguous) rows (namely, at most one row for each choice of $0\le x<\til{y}_0$, $R\in\{A,\bar{B}\}$, 
and $\alpha\in\req_R\bigl(\cL(x,\til{y}_0)\bigr)$). We call \emph{gap} of $\img_y(f)$ any set $Y=\{y,y+1,...,y'\}$ 
of contiguous rows of $\cG$ such that $\til{y}_0<y \leq y' < \max\bigl(\img_y(f)\bigr)$ and $\img_y(f)\cap Y=\emptyset$. 
From previous results (in particular, from the proofs of Lemma \ref{lemma:contraction_finite} and Theorem 
\ref{th:contraction_finite}), we can assume, without loss of generality, that every gap $Y$ of $\img_y(f)$ 
has size at most $2^{2^{7\len{\varphi}}}-1$ (otherwise, we can find two rows $y'_0$ and $y'_1$ in $Y$ that 
satisfy the hypothesis of Lemma \ref{lemma:contraction_finite} and hence we can ``remove'' the rows from 
$y'_0$ to $y'_1-1$ from $\cG$, without affecting consistency and fulfillment). This shows that 
$\max\bigl(\img_y(f)\bigr)$ $\le$ $\til{y}_0 + 2\len{\varphi}\cdot\til{y}_0\cdot 2^{2^{7\len{\varphi}}}$.
We then define $\til{y}$ as the least value such that $\til{y}_0\til{y}>\max\bigl(\img_y(f)\bigr)$ and 
$\shading_\cG(\til{y}_0)=\shading_\cG(\til{y}_0+\til{y})$. Again, by exploiting simple counting arguments, 
one can prove that 
$\til{y}$ $<$ $\max\bigl(\img_y(f)\bigr) - \til{y}_0 + 2^{2^{7\len{\varphi}}}$ 
        $\le$ $2\len{\varphi}\cdot\til{y}_0\cdot 2^{2^{7\len{\varphi}}} + 2^{2^{7\len{\varphi}}}$
        $\le$ $\bigl(2\len{\varphi}\cdot\til{y}_0+1\bigr)\cdot 2^{2^{7\len{\varphi}}}$
        $\le$ $2 \len{\varphi}\cdot\bigl(\til{y}_0+1\bigr)\cdot 2^{2^{7\len{\varphi}}}$
        $\le$ $2 \len{\varphi}\cdot 2^{2^{7\len{\varphi}}}\cdot 2^{2^{7\len{\varphi}}}$.

\smallskip\noindent
\textsc{Binding $\til{g}$.\;\;}
Since $\shading_\cG(\til{y}_0)=\shading_\cG(\til{y}_0+\til{y})$, we know that there is a (surjective) 
function $g$ that maps any value $x\in\{0,...,\til{y}_0+\til{y}-1\}$ to a value $g(x)\in\{0,...,\til{y}_0-1\}$ 
in such a way that $\cL(x,\til{y}_0+\til{y})=\cL(g(x),\til{y}_0)$. We choose
one such function as $\til{g}$. 

\smallskip\noindent
\textsc{Periodic compass structure $\cG'$.\;\;} 
According to Definition \ref{def:periodiccompassstructure}, the threshold $\til{y}_0$, the period 
$\til{y}$, the binding $\til{g}$, and the labeling $\cL$ of $\cG$ restricted to the finite domain
$\bbP_{\til{y}_0+\til{y}-1}$ uniquely determine a periodic structure $\cG'=(\bbP_\omega,\cL')$.
It thus remains to show that $\cG'$ is a (consistent and fulfilling) compass structure that 
features $\varphi$. The proof that the labeling $\cL'$ is consistent with the relations $A$, $B$, 
and $\bar{B}$ is straightforward, given the above construction. As for the fulfillment of the 
various requests, one can prove, by induction on $n$, that, for every $n\in\bbN$, every point 
$p=(x,y)$ with $y=\til{y}_0+n\til{y}$, every relation $R\in\{A,\bar{B}\}$ (resp., $R=B$), and 
every $R$-request $\alpha\in\req_R\bigl(\cL'(p)\bigr)$, there is a point $p'=(x',y')$ such 
that $y'\le\til{y}_0+(n+1)\til{y}$ (resp., $y'< \til{y}_0+n\til{y}$), $p \;R\; p'$, and 
$\alpha\in\obs\bigl(\cL'(p')\bigr)$. This suffices to claim that $\cG'$ is a consistent and 
fulfilling compass structure. Consider the case of relation $\bar{B}$ (the case of relation
$B$ is fully symmetric and the case of relation $A$ can be easily reduced to that of $\bar{B}$). 
By contradiction, let us suppose that there is a point $p=(x,y)$, with $\til{y}_0+n\til{y}<y<\til{y}_0+(n+1)\til{y}$, 
such that $\alpha\in\req_{\bar{B}}\bigl(\cL(p)\bigr)$ and $\alpha\nin\obs\bigl(\cL(p')\bigr)$ 
for all points $p'$ such that $p \;\bar{B}\; p'$. Since $\cG'$ is consistent, we have 
$\alpha\in\req_{\bar{B}}\bigl(\cL(q)\bigr)$, where $q=\bigl(x,\til{y}_0+(n+1)\til{y}\bigr)$
(note that $p \;\bar{B}\; q$ holds) and thus, by construction, there is a point $q'=(x,y')$, 
with $\til{y}_0+(n+1)\til{y}<y'\le\til{y}_0+(n+2)\til{y}$, such that $\alpha\in\obs\bigl(\cL(q')\bigr)$ 
(a contradiction). Finally, one can show that $\cG'$ features the formula $\varphi$ by exploiting the 
same argument that was given in the proof of Lemma \ref{lemma:contraction_finite}.
\end{proof}

\subsection{Proof of Lemma \ref{lemma:hardness}}\label{app:hardness}

\smallskip\noindent
{\bf Lemma \ref{lemma:hardness}.}
\emph{
There is a polynomial-time reduction from the exponential-corridor tiling problem 
to the satisfiability problem for $\ABB$.
}
\medskip

\begin{figure}[!tb]
\centering
\includegraphics{draft.4}
\caption{Encoding of a tiling function.}
\label{fig:tiling}
\end{figure}
\begin{proof}
Consider a generic instance $\cT=(T,t_\bot,t_\top,H,V,n)$ of the exponential-corridor tiling problem,
where $T=\{t_1,\ldots,t_k\}$. We guarantee the existence of a tiling function $f:\bbN\times\{0,...,2^n-1\}\then T$ 
that satisfies the instance $\cT$ through the existence of a labeled (infinite) interval structure 
$\cS=(\bbI_\omega,A,B,\sigma)$ that satisfies a suitable $AB$ formula with size polynomial in $\cT$. 
We use $k$ propositional variables $t_1,...,t_k$ to represent the tiles from $T$,
$n$ propositional variables $y_0,...,y_{n-1}$ to represent the binary expansion of the $y$-coordinate 
of a row, and one propositional variable $c$ to identify those intervals in $\bbI_\omega$ that correspond 
to points of the infinite corridor of height $2^n$. The correspondence between the points $p=(x,y)$, 
with $x\in\bbN$ and $0\le y<2^n$, of the infinite corridor and the intervals $I_p\in\bbI_\omega$ 
is obtained by letting $I_p=[y+2^n x,y+2^n x+1]$ (Figure \ref{fig:tiling} can be used as a reference example
through the rest of the proof). According to such an encoding, the labeling function $\sigma$ is related to 
the tiling function $f$ as follows:

\bigskip
\begin{center}
\parbox{13cm}{\emph{for every point $p=[x,y]\in\bbN\times\{0,...,2^n-1\}$ and every index $1\le i\le k$, 
                    if $f(p)=t_i$, then $\sigma(I_p)=\{c,t_i,y_{j_1},...,y_{j_h}\}$, where 
                    $\{j_1,...,j_j\}\subseteq\{0,...,n-1\}$ and $y=\sum_{j\in\{j_1,...,j_h\}}2^j$.}}
\end{center}
\bigskip

\noindent
For the sake of brevity, we introduce a universal modal operator $\BU$, which is defined as follows:
$$
  \BU\alpha \,=\, \alpha \,\et\, \BA \alpha \,\et\, \BA\BA \alpha.
$$
We now show how to express the existence of a tiling function $f$ that satisfies $\cT$. First of all, we 
associate the propositional variable $c$ with all and only the intervals of the form $I_p=[y+2^n x,y+2^n 
x+1]$, with $x\in\bbN$ and $0\le y<2^n$ (atomic intervals), as follows:
$$
  \varphi_c \,=\, \BU(c \iff \BB\bot).
$$
The tiling function $f:\bbN\times\{0,...,2^n-1\}\then T$ is represented by associating with each 
$c$-labeled interval $I_p=[y+2^n x,y+2^n x+1]$ a unique propositional variable $f(p)$ in $T$ as follows:
$$
  \varphi_f \,=\, \BU\left(c \then \bigvee\nolimits_{1\le i\le k}t_i\right) \;\et\; \BU\left(c \then \bigwedge\nolimits_{1\le i<j\le k} \neg(t_i \et t_j)\right).
$$
Next, we associate with each (possibly non-minimal) interval of the form $I=[y+2^n x,y+2^n x+l]$ a subset of 
the propositional variables $y_0,...,y_{n-1}$ that encodes the binary expansion of $y$. Such a labeling 
can be enforced by the formula:
$$
  \varphi_y \,=\, \Bigl(\bigwedge\nolimits_{0\le i<n}\!\neg y_i\Bigr) \,\et\,
                  \BU\Bigl(\bigwedge\nolimits_{0\le i<n}\!\bigl(y_i \!\!\iff\!\! \BB y_i\bigr) \et \bigl(\neg y_i \!\!\iff\!\! \BB \neg y_i\bigr)\Bigr) \,\et\,
                  \BU\Bigl(c \!\!\then\!\! \varphi^0_{\mit{inc}}\Bigr)
$$
where the formula $\varphi^i_{\mit{inc}}$ is defined (by induction on $i\in\{n,...,0\}$) as follows:
$$
\begin{array}{rcl}
  \varphi^i_{\mit{inc}} &=& \begin{cases}
                              \top                                                                                                           & \text{if $i=n$,}    \s1 \\
                              \Bigl(y_i \!\et\! \DA(c \!\!\et\!\! \neg y_i) \!\et\! \varphi^{i+1}_{\mit{inc}}\Bigr) \,\vel\,    
                              \Bigl(\neg y_i \!\et\! \DA(c \!\!\et\!\! y_i) \!\et\! \varphi^{i+1}_{\mit{eq}}\Bigr)                           & \text{if $i<n$,}
                            \end{cases}
\end{array}
$$
The formula $\varphi^i_{\mit{inc}}$ involves the formula $\varphi^i_{\mit{eq}}$, which 
is defined (by induction on $i\in\{n,...,0\}$) as follows:

$$
\begin{array}{rcl}                                               
  \varphi^i_{\mit{eq}}  &=& \begin{cases}
                              \top                                                                                                           & \quad\quad\,\,\text{if $i=n$,}    \s1 \\
                              \Bigl(\bigl(y_i \et \DA(c \!\!\et\!\! y_i)\bigr) \,\vel\, \bigl(\neg y_i \et \DA(c \!\!\et\!\! \neg y_i)\Bigl) \,\et\,
                              \varphi^{i+1}_{\mit{eq}}                                                                                       & \quad\quad\,\,\text{if $i<n$.}
                            \end{cases}
\end{array}
$$
It remains to express the constraints on the tiling function $f$. This can be done by using the following formulas
(for the sake of simplicity, we assume, without loss of generality, that $(t_\top,t_\bot)\in V$):
$$
\begin{array}{rcl}
  \varphi_\bot &=& \BU\Bigr(c \et \bigwedge\nolimits_{0\le i<n}\neg y_i \;\then\; t_\bot\Bigr)   \s3 \\
  \varphi_\top &=& \BU\Bigr(c \et \bigwedge\nolimits_{0\le i<n}y_i \;\then\; t_\top\Bigr)        \s3 \\
  \varphi_H    &=& \BU\bigwedge\nolimits_{1\le i\le k}\Bigl(\bigl(\varphi_{\mit{corr}} \et \DB(c \et t_i)\bigr) \then \bigvee\nolimits_{(t_i,t_j)\in H} \DA(c \et t_j)\Bigr)   \s3 \\
  \varphi_V    &=& \BU\bigwedge\nolimits_{1\le i\le k}\Bigl((c \et t_i) \then \bigvee\nolimits_{(t_i,t_j)\in V} \DA(c \et t_j)\Bigr),
\end{array}
$$
where $\varphi_{\mit{corr}}=\varphi^0_{\mit{eq}} \et \BB\neg\varphi^0_{\mit{eq}}$ (intuitively, 
the formula $\varphi_{\mit{corr}}$ holds over all and only the intervals of the form 
$I=\bigl[y+2^n x,y+2^n(x+1)\bigr]$, in such a way that, if $J$ and $K$ are the shortest 
intervals such that $I \;B\; J$ and $I \;A\; K$, then $J$ corresponds to the point $p=(x,y)$ 
and $K$ corresponds to the point $q=(x+1,y)$).

\smallskip\noindent
Summing up, we have that the formula $\varphi \,=\, \varphi_c \et \varphi_f \et \varphi_y \et \varphi_\bot \et \varphi_\top \et \varphi_H \et \varphi_V$,
which has polynomial size in $\len{\cT}$ and uses only the modal operators $\DA$ and $\DB$, is satisfiable if and only if $\cT$ is a positive instance of 
the exponential-corridor tiling problem.
\end{proof}

\subsection{Proof of Lemma \ref{lemma:completeness}}\label{app:completeness}

\smallskip\noindent
{\bf Lemma \ref{lemma:completeness}.}
\emph{
There is an EXPSPACE non-deterministic procedure that decides whether a given formula 
of $\ABB$ is satisfiable or not.
}
\bigskip

In order to prove this lemma, we need to introduce two variants of the dependency relations $\dep{B}$
and $\dep{A}$, which are more restrictive than the previous ones and which are evaluated (locally)
over pairs of atoms that lie along two contiguous rows. Precisely, we define the following relations 
between atoms $F$ and $G$:
$$
\begin{array}{rcl}
  F \localdep{A} G    
  &\;\quad\text{iff}\quad\quad&   
  \begin{cases}   
    \req_A(F)                                              \;=\;          \obs(G) \,\cup\, \req_{\bar{B}}(G)    \s1 \\
    \req_B(G)                                              \;=\;          \emptyset
  \end{cases}                                                                                                   \s2 \\
  F \localdep{B} G    
  &\;\quad\text{iff}\quad\quad&   
  \begin{cases}   
    \req_B(F)                                              \;=\;          \obs(G) \,\cup\, \req_B(G)            \s1 \\
    \req_{\bar{B}}(G)                                      \;=\;          \obs(F) \,\cup\, \req_{\bar{B}}(F).
  \end{cases}
\end{array}
$$
Note that $F\localdep{A}G$ (resp., $F\localdep{B}G$) implies $F\dep{A}G$ (resp., $F\dep{B}G$),
but the converse implications are not true in general. Moreover, it is easy to see that any 
consistent and fulfilling finite compass structure $\cG=(\bbI_N,\cL)$, with $N\in\bbN$, satisfies 
the following properties, and, conversely, any finite structure $\cG=(\bbI_N,\cL)$, with $N\in\bbN$,
that satisfies the following properties is a consistent and fulfilling compass structure:
\begin{romlist}
  \item for every pair of points $p=(x,y)$ and $q=(y,y+1)$ in $\cG$, we have $\cL(p)\localdep{A}\cL(q)$,
  \item for every pair of points $p=(x,y)$ and $q=(x,y+1)$ in $\cG$, we have $\cL(q)\localdep{B}\cL(p)$,
  \item for the lower-left point $p=(0,1)$ in $\cG$, we have $\req_B\bigl(\cL(p)\bigr)=\emptyset$,
  \item for every upper point $p=(x,N)$ in $\cG$, we have $\req_{\bar{B}}\bigl(\cL(p)\bigr)=\emptyset$
        and $\req_A\bigl(\cL(p)\bigr)=\emptyset$.
\end{romlist}

\bigskip
Now, we can prove Lemma \ref{lemma:completeness}.
\medskip

\begin{proof}
We first consider the (easier) case of satisfiability with interpretation over finite interval 
structures; then, we shall deal with the more general case of satisfiability with interpretation
over infinite interval structures. 

\small

\begin{figure}[!!tb]
\centering
\begin{code}
  \LET \varphi \text{ be an input formula} \s3 \\
  
  \PROCEDURE{CheckConsistency}{S,f,\ort{G}}
  \BEGIN
    \FOREACH \text{$\varphi$-atom } F\in S \DO
    \BEGIN
      \IF F\nlocaldep{A}\ort{G} \OR f(F)\nlocaldep{B}F \THEN
        \RETURN{\FALSE}
    \END \\
    \RETURN{\TRUE}
  \END
  \ENDPROCEDURE
    
  \PROCEDURE{CheckFulfillment}{S}
  \BEGIN
    \FOREACH \text{$\varphi$-atom } F\in S \DO
    \BEGIN
      \IF \req_{A}(F)\neq\emptyset \OR \req_{\bar{B}}(F)\neq\emptyset \THEN
        \RETURN{\FALSE}
    \END \\
    \RETURN{\TRUE}
  \END
  \ENDPROCEDURE
  
  \MAIN
  \BEGIN
    N \GETS \text{ any value in } \bigl\{1,...,2^{2^{7\len{\varphi}}}\bigr\} \\  
    F \GETS \text{ any $\varphi$-atom such that $\req_B(F)=\emptyset$ and $\varphi\in\obs(F)\cup\req_{\bar{B}}(F)$} \\ 
    S \GETS \{F\} \\ 
    
    \FOR y \GETS 1 \TO N \DO                                                    
    \BEGIN
      f \GETS \text{ any mapping from $S$ to the set of all $\varphi$-atoms} \\
      \ort{G} \GETS \text{ any $\varphi$-atom} \\
      \IF \NOT \CALL{CheckConsistency}{S,g,\ort{G}} \THEN
        \RETURN{\FALSE} \\
      S \GETS \bigl\{f(F) \,:\, F\in S\bigr\} \cup \bigl\{\ort{G}\bigr\}
    \END \s2 \\
    
    \RETURN{\ \CALL{CheckFulfillment}{S}}
  \END
  \ENDMAIN
\end{code}
\caption{Algorithm for the satisfiability problem over finite structures.}
\label{fig:completeness_finite}
\end{figure}
\normalsize
\smallskip\noindent
\textsc{Finite case.\;\;}
In Figure \ref{fig:completeness_finite}, we describe an EXPSPACE non-deterministic procedure that 
decides whether a given $\ABB$ formula is satisfiable over finite labeled interval structures. 
Below, we prove that such a procedure is sound and complete. 

\smallskip\noindent
\textsc{(Soundness)\;\;}
As for the soundness, we consider a successful computation of the procedure and we show that there 
is a finite compass structure $\cG=(\bbP_N,\cL)$ that features $\varphi$, where $N\in\bbN$ is exactly 
the value that was guesses at the beginning of the computation. We build such a structure $\cG$ 
inductively on the value of the variable $y\in\{1,...,N\}$ as follows.
\begin{dotlist}
  \item If $y=1$, then we let $\cG_1=(\bbI_1,\cL_1)$, where $\cL_1$ maps the unique point of $\bbI_1$ 
        to the atom $F$ that was guessed at the beginning of the computation. Note that $\cG_1$ satisfies 
        the consistency condition of Definition \ref{def:compassstructure}, but it may not satisfy the 
        fulfillment condition for the relations $A$ and $\bar{B}$.
  \item If $y>1$, then assuming that $\cG_{y-1}=(\bbI_{y-1},\cL_{y-1})$ is the consistent (possibly 
        non-fulfilling) compass structure obtained during the $y-1$-th iteration, we define 
        $\cG_y=(\bbI_y,\cL_y)$, where:
        \begin{romlist}
          \item $\cL_y(p)=\cL_{y-1}(p)$ for every point $p=(x',y')$ that belongs to $\bbI_{y-1}$, 
                namely, such that $0\le x'<y'<y$;
          \item $\cL_y(p)=f\bigl(\cL_{y-1}(q)\bigr)$ for every pair of points of the form $p=(x,y)$ 
                and $q=(x,y-1)$, with $0\le x<y-1$, where $f$ is the function guessed during the 
                $y$-th iteration;
          \item $\cL_y(\ort{p})=\ort{G}$, where $\ort{p}=(y-1,y)$ and $\ort{G}$ is the atom guessed 
                during the $y$-th iteration.
        \end{romlist}
\end{dotlist}
We then define $\cG$ to be the structure $\cG_N$. Now, knowing that every call to the function 
{\bf\textsc{CheckConsistency}} was successful, we can conclude that the structure $\cG$ satisfies
the following two properties:
\begin{romlist}
  \item for every pair of points $p=(x,y)$ and $q=(y,y+1)$ in $\cG$, we have $\cL(p)\localdep{A}\cL(q)$,
  \item for every pair of points $p=(x,y)$ and $q=(x,y+1)$ in $\cG$, we have $\cL(q)\localdep{B}\cL(p)$.
\end{romlist}
Moreover, since the first guessed atom $F$ was such that $\req_B(F)=\emptyset$ and since the call 
to the function {\bf\textsc{CheckFulfillment}} at the end of the computation was successful, we know 
that $\cG$ satisfies also the following two properties:
\begin{romlist}
  \addtocounter{enumi}{2}
  \item for the lower-left point $p=(0,1)$, we have $\req_B\bigl(\cL(p)\bigr)=\emptyset$,
  \item for every upper point $p=(x,N)$, we have $\req_{\bar{B}}\bigl(\cL(p)\bigr)=\emptyset$
        and $\req_A\bigl(\cL(p)\bigr)=\emptyset$.
\end{romlist}
By previous arguments, this shows that $\cG$ is a consistent and fulfilling compass structure.
Finally, since the first guessed atom $F$ was such that $\varphi\in\obs(F)\cup\req_{\bar{B}}(F)$, 
we have that $\cG$ features the input formula $\varphi$. Proposition \ref{prop:compassstructure} 
finally implies that there is a labeled finite interval structure that satisfies $\varphi$.

\smallskip\noindent
\textsc{(Completeness)\;\;}
As for completeness, we consider a finite labeled interval structure $\cS=(\bbI_{N'},A,B,\bar{B},\sigma)$ 
that satisfies $\varphi$. By Theorem \ref{th:contraction_finite}, we know that there is a (consistent 
and fulfilling) compass structure $\cG=(\bbI_N,\cL)$ of length $N\le 2^{2^{7\len{\varphi}}}$ that features 
$\varphi$. We exploit such a structure $\cG$ to show that there is a successful computation of the 
algorithm of Figure \ref{fig:completeness_finite}. To do that, it is sufficient to describe, at each step 
of the computation where the value of a variable needs to be guessed, which is the right choice for that
value. Clearly, at the beginning of the computation, the variable $N$ will take as value exactly the 
length of the compass structure $\cG$. Similarly, the initial value for the variable $F$ is chosen to 
be the atom $\bigl\{\cL(p)\bigr\}$ associated with the lower-left point $p=(0,1)$. Then, at each iteration 
of the main loop, we choose the values for $f$ and for $\ort{G}$ as follows. We assume that, at the $y$-th 
iteration, $S$ is exactly the shading associated with the row $y$ in $\cG$ (it can be easily proved that 
this is an invariant of the computation) and, for every atom $F$ in $S$, we denote by $p_F=(x_F,y)$ a 
generic point along the row $y$ such that $\cL(p_F)=F$ (such a point exists by assumption). We then choose 
$f$ to be the function that maps every atom $F\in S$ to the atom $f(F)=\cL(x_F,y+1)$. It is routine to 
prove that the computation that results from the above-defined sequence of guesses is successful.

\small

\begin{figure}[!!tb]
\centering
\begin{code}
  \LET \varphi \text{ be an input formula} \s2 \\
  
  \PROCEDURE{CheckConsistency}{S,f,\ort{G}}
    \text{\emph{(as before)}}\vspace{-2mm}
  \ENDPROCEDURE
    
  \PROCEDURE{UpdateFulfillment}{\mit{fulfilled},\til{S},\til{f},S,\ort{G}}
  \BEGIN
    \FOREACH \text{$\varphi$-atom } F\in\til{S} \text{ and $A$-request }\alpha\in\req_A(F) \DO
    \BEGIN
      \IF \alpha\in\obs(\ort{G}) \THEN
        \mit{fulfilled}[F,A,\alpha] \GETS \TRUE
    \END \\
    \FOREACH \text{$\varphi$-atom } F\in\til{S} \text{ and $\bar{B}$-request }\alpha\in\req_{\bar{B}}(F) \DO
    \BEGIN
      \IF \alpha\in\obs(\til{f}(F)) \THEN
        \mit{fulfilled}[F,\bar{B},\alpha] \GETS \TRUE
    \END
  \END\vspace{-0.5mm}
  \ENDPROCEDURE
  
  \PROCEDURE{CheckFulfillment}{\mit{fulfilled},\til{S},\til{f},S}
  \BEGIN
    \IF S\neq\til{S} \THEN
      \RETURN{\FALSE} \\
    \FOREACH \text{$\varphi$-atom } F\in\til{S}, \text{ relation } R\in\{A,\bar{B}\}, \text{ and $R$-request }\alpha\in\req_R(F) \DO
    \BEGIN
      \IF \NOT \mit{fulfilled}[F,R,\alpha] \THEN
        \RETURN{\FALSE}
    \END \\
    \RETURN{\TRUE}
  \END\vspace{-0.5mm}
  \ENDPROCEDURE
  
  \MAIN
  \BEGIN
    \til{y}_0 \GETS \text{ any value in } \bigl\{1,...,2^{2^{7\len{\varphi}}-1}\bigr\} \\  
    \til{y} \GETS \text{ any value in } \bigl\{1,...,2\len{\varphi}\cdot 2^{2^{7\len{\varphi}}}\cdot 2^{2^{7\len{\varphi}}}-1\bigr\} \\  
    F \GETS \text{ any $\varphi$-atom such that $\req_B(F)=\emptyset$ and $\varphi\in\obs(F)\cup\req_{\bar{B}}(F)$} \\ 
    S \GETS \{F\} \s1 \\ 
    
    \FOR y \GETS 1 \TO \til{y}_0 \DO                                                    
    \BEGIN
      f \GETS \text{ any mapping from $S$ to the set of all $\varphi$-atoms} \\
      \ort{G} \GETS \text{ any $\varphi$-atom} \\
      \IF \NOT \CALL{CheckConsistency}{S,g,\ort{G}} \THEN
        \RETURN{\FALSE} \\
      S \GETS \bigl\{f(F) \,:\, F\in S\bigr\} \cup \bigl\{\ort{G}\bigr\}
    \END \s1 \\
    
    \til{S} \GETS S \\
    \til{f} \GETS \text{ the identity function on $\til{S}$} \\
    \FOREACH \text{$\varphi$-atom } F\in\til{S}, \text{ relation } R\in\{A,\bar{B}\}, \text{ and $R$-request }\alpha\in\req_R(F) \DO
      \mit{fulfilled}[F,R,\alpha] \GETS \FALSE \s1 \\
    
    \FOR y \GETS \til{y}_0+1 \TO \til{y}_0+\til{y} \DO                                                    
    \BEGIN
      f \GETS \text{ any mapping from $S$ to the set of all $\varphi$-atoms} \\
      \ort{G} \GETS \text{ any $\varphi$-atom} \\
      \IF \NOT \CALL{CheckConsistency}{S,g,\ort{G}} \THEN
        \RETURN{\FALSE} \\
      \til{f} \GETS f\circ\til{f} \\
      S \GETS \bigl\{f(F) \,:\, F\in S\bigr\} \cup \bigl\{\ort{G}\bigr\} \\
      \CALL{UpdateFulfillment}{\mit{fulfilled},\til{S},\til{f},S,\ort{G}}
    \END \s2 \\

    \RETURN{\ \CALL{CheckFulfillment}{\mit{fulfilled},\til{S},\til{f},S}}
    \END
  \ENDMAIN
\end{code}
\caption{Algorithm for the satisfiability problem over infinite structures.}
\label{fig:completeness_infinite}
\end{figure}
\normalsize
\smallskip\noindent
\textsc{Infinite case.\;\;}
Figure \ref{fig:completeness_infinite} reports an EXPSPACE non-deterministic procedure that 
decides whether a given $\ABB$ formula is satisfiable over infinite labeled interval structures. 

\smallskip\noindent
\textsc{(Soundness)\;\;}
In order to prove that the described procedure is sound, we consider a successful computation 
of the procedure and we show that there is an infinite periodic compass structure $\cG=(\bbP_\omega,\cL)$ 
that features $\varphi$. The threshold $\til{y}_0$ and the period $\til{y}$ of $\cG$ are defined 
to be the values of the corresponding variables that were guessed at the beginning of the computation. 
As for the binding function $\til{g}$, we choose any arbitrary mapping $\til{g}$ from $S$ to $\til{S}$ 
such that $\til{g}\circ\til{f}$ is the identity on $S$, where $S$, $\til{S}$, and $\til{f}$ are the 
values of the corresponding variables at the end of the computation. It now remains to describe the 
labeling of the finite portion $\bbP_{\til{y}_0+\til{y}-1}$ of $\cG$ (note that this labeling uniquely 
determines the infinite periodic compass structure $\cG$). This can be done by following the same 
construction given in the finite case. Similarly, the fact that $\cG$ satisfies the consitency 
conditions of Definition \ref{def:compassstructure} can be proved by exploiting arguments analogous 
to the finite case. The proof that $\cG$ satisfies also the fulfillment condition requires more
details. In particular, one can prove, again by exploiting induction on $y$, that for every 
row $y$, with $\til{y}_0\le y<\til{y}_0+\til{y}$, every point $p=(x,\til{y}_0)$, every relation 
$R\in\{A,\bar{B}\}$, and every $R$-request $\alpha\in\req_R\bigl(\cL(p)\bigr)$, if $\cL(p)=F$ 
($\in\til{S}$) and $\mit{fulfilled}[F,R,\alpha]$ is true during the $y$-th iteration of the 
main loop, then there exists a point $q=(x',y)$ such that $p \;R\; q$ and $\alpha\in\obs\bigl(\cL(q)\bigr)$.
Thus, at the end of the computation, since all entries of the variable $\mit{fulfilled}$
are set to {\bf\textsc{true}}, we know that all $A$-requests and all $\bar{B}$-requests
of atoms associated with row $\til{y}_0$ are fulfilled below row $\til{y}_0+\til{y}$.
This shows that $\cG$ is a consistent and fulfilling compass structure. As before, one
can conclude that $\cG$ features the input formula $\varphi$ and hence there exists
an infinite labeled interval structure that satisfies $\varphi$.

\smallskip\noindent
\textsc{(Completeness)\;\;}
As for completeness, we consider an infinite labeled interval structure $\cS=(\bbI_\omega,A,B,\bar{B},\sigma)$
that satisfies $\varphi$. By Theorem \ref{th:contraction_infinite}, we know that there is a periodic 
(consistent and fulfilling) compass structure $\cG=(\bbI_\omega,\cL)$, with threshold 
$\til{y}_0<2^{2^{7\len{\varphi}}}$, period $\til{y}<2\len{\varphi}\cdot 2^{2^{7\len{\varphi}}}\cdot 2^{2^{7\len{\varphi}}}$, 
and binding $\til{g}:\{0,...,\til{y}_0+\til{y}-1\}\then\{0,...,\til{y}_0-1\}$. We exploit
such a periodic structure $\cG$ to show that there is a successful computation of the algorithm 
of Figure \ref{fig:completeness_infinite}. In particular, at each step of the computation where 
the value of a variable needs to be guessed, we describe which is the right choice for that value. 
Clearly, at the beginning of the computation, the variables $\til{y}_0$ and $\til{y}$ will take 
as values exactly the threshold and the period of the compass structure $\cG$. Similarly, the 
initial value for the variable $F$ is chosen to be the atom $\bigl\{\cL(p)\bigr\}$ associated 
with the lower-left point $p=(0,1)$. Then, at each iteration of one of the two main loops, we 
choose the values for $f$ and for $\ort{G}$ as follows. We assume that, at each iteration of
one of the two loops, $S$ is the shading associated with the row $y$ in $\cG$, where $y$ is
the value of the corresponding variable (it can be easily proved that this is an invariant of 
the computation) and, for every atom $F$ in $S$, we denote by $p_F=(x_F,y)$ a generic point 
along the row $y$ such that $\cL(p_F)=F$ (such a point exists by assumption). We then choose 
$f$ to be the function that maps every atom $F\in S$ to the atom $f(F)=\cL(x_F,y+1)$. It is 
routine to prove that the computation that results from the above-defined sequence of guesses 
is successful.
\end{proof}
